# Supplementary material for: End-to-End Deep Structured Models for Drawing Crosswalks
Source: arXiv:2012.11585 source file (2021-01-14)
Supplement: Supplementary file 1 [file results_vis.tex]

%!TEX root = evaluation.tex

\begin{figure}
\begin{tabular}{cccccccr}
\includegraphics[width=.1595\textwidth]{images/results/{0.9335_sfo_b1117462-6815-46a9-c57a-5004fc3af792_788e49e7-ca7a-43a7-c1a6-fa36ba6ab3db_ground}.png} &
\includegraphics[width=.1595\textwidth]{images/results/{0.9335_sfo_b1117462-6815-46a9-c57a-5004fc3af792_788e49e7-ca7a-43a7-c1a6-fa36ba6ab3db_lidar}.png} &
\includegraphics[width=.1595\textwidth]{images/results/{0.9335_sfo_b1117462-6815-46a9-c57a-5004fc3af792_788e49e7-ca7a-43a7-c1a6-fa36ba6ab3db_dt}.png} &
\includegraphics[width=.1595\textwidth]{images/results/{0.9335_sfo_b1117462-6815-46a9-c57a-5004fc3af792_788e49e7-ca7a-43a7-c1a6-fa36ba6ab3db_seg}.png} &
\includegraphics[width=.1595\textwidth]{images/results/{0.9335_sfo_b1117462-6815-46a9-c57a-5004fc3af792_788e49e7-ca7a-43a7-c1a6-fa36ba6ab3db_inf_pred}.png} &
\includegraphics[width=.1595\textwidth]{images/results/{0.9335_sfo_b1117462-6815-46a9-c57a-5004fc3af792_788e49e7-ca7a-43a7-c1a6-fa36ba6ab3db_inf_gt}.png} &\\

\includegraphics[width=.1595\textwidth]{images/results/{0.9011_sfo_4e0ec985-25b7-41e5-f557-be65ad442d6e_732ef14c-b8ee-4e25-eb5f-a6f3f6574313_ground}.png} &
\includegraphics[width=.1595\textwidth]{images/results/{0.9011_sfo_4e0ec985-25b7-41e5-f557-be65ad442d6e_732ef14c-b8ee-4e25-eb5f-a6f3f6574313_lidar}.png} &
\includegraphics[width=.1595\textwidth]{images/results/{0.9011_sfo_4e0ec985-25b7-41e5-f557-be65ad442d6e_732ef14c-b8ee-4e25-eb5f-a6f3f6574313_dt}.png} &
\includegraphics[width=.1595\textwidth]{images/results/{0.9011_sfo_4e0ec985-25b7-41e5-f557-be65ad442d6e_732ef14c-b8ee-4e25-eb5f-a6f3f6574313_seg}.png} &
\includegraphics[width=.1595\textwidth]{images/results/{0.9011_sfo_4e0ec985-25b7-41e5-f557-be65ad442d6e_732ef14c-b8ee-4e25-eb5f-a6f3f6574313_inf_pred}.png} &
\includegraphics[width=.1595\textwidth]{images/results/{0.9011_sfo_4e0ec985-25b7-41e5-f557-be65ad442d6e_732ef14c-b8ee-4e25-eb5f-a6f3f6574313_inf_gt}.png} &\\

\includegraphics[width=.1595\textwidth]{images/results/{0.9310_sfo_9ecb3b4e-78fc-4e68-de47-4a269e205d2a_4db38371-47b3-4d76-ca5e-a0e216848f7b_ground}.png} &
\includegraphics[width=.1595\textwidth]{images/results/{0.9310_sfo_9ecb3b4e-78fc-4e68-de47-4a269e205d2a_4db38371-47b3-4d76-ca5e-a0e216848f7b_lidar}.png} &
\includegraphics[width=.1595\textwidth]{images/results/{0.9310_sfo_9ecb3b4e-78fc-4e68-de47-4a269e205d2a_4db38371-47b3-4d76-ca5e-a0e216848f7b_dt}.png} &
\includegraphics[width=.1595\textwidth]{images/results/{0.9310_sfo_9ecb3b4e-78fc-4e68-de47-4a269e205d2a_4db38371-47b3-4d76-ca5e-a0e216848f7b_seg}.png} &
\includegraphics[width=.1595\textwidth]{images/results/{0.9310_sfo_9ecb3b4e-78fc-4e68-de47-4a269e205d2a_4db38371-47b3-4d76-ca5e-a0e216848f7b_inf_pred}.png} &
\includegraphics[width=.1595\textwidth]{images/results/{0.9310_sfo_9ecb3b4e-78fc-4e68-de47-4a269e205d2a_4db38371-47b3-4d76-ca5e-a0e216848f7b_inf_gt}.png} &\\

\includegraphics[width=.1595\textwidth]{images/results/{0.9278_sfo_150ad5e5-4d6a-44c2-d8c5-eea4ab66f009_9bb369d6-fc48-48fa-e437-ea240ab2d72c_ground}.png} &
\includegraphics[width=.1595\textwidth]{images/results/{0.9278_sfo_150ad5e5-4d6a-44c2-d8c5-eea4ab66f009_9bb369d6-fc48-48fa-e437-ea240ab2d72c_lidar}.png} &
\includegraphics[width=.1595\textwidth]{images/results/{0.9278_sfo_150ad5e5-4d6a-44c2-d8c5-eea4ab66f009_9bb369d6-fc48-48fa-e437-ea240ab2d72c_dt}.png} &
\includegraphics[width=.1595\textwidth]{images/results/{0.9278_sfo_150ad5e5-4d6a-44c2-d8c5-eea4ab66f009_9bb369d6-fc48-48fa-e437-ea240ab2d72c_seg}.png} &
\includegraphics[width=.1595\textwidth]{images/results/{0.9278_sfo_150ad5e5-4d6a-44c2-d8c5-eea4ab66f009_9bb369d6-fc48-48fa-e437-ea240ab2d72c_inf_pred}.png} &
\includegraphics[width=.1595\textwidth]{images/results/{0.9278_sfo_150ad5e5-4d6a-44c2-d8c5-eea4ab66f009_9bb369d6-fc48-48fa-e437-ea240ab2d72c_inf_gt}.png} &\\

\includegraphics[width=.1595\textwidth]{images/results/{0.9354_sfo_df2a4d5e-6476-40f1-d0a9-898828e1593e_312de068-0f7b-407c-fa9c-88f7447b20ed_ground}.png} &
\includegraphics[width=.1595\textwidth]{images/results/{0.9354_sfo_df2a4d5e-6476-40f1-d0a9-898828e1593e_312de068-0f7b-407c-fa9c-88f7447b20ed_lidar}.png} &
\includegraphics[width=.1595\textwidth]{images/results/{0.9354_sfo_df2a4d5e-6476-40f1-d0a9-898828e1593e_312de068-0f7b-407c-fa9c-88f7447b20ed_dt}.png} &
\includegraphics[width=.1595\textwidth]{images/results/{0.9354_sfo_df2a4d5e-6476-40f1-d0a9-898828e1593e_312de068-0f7b-407c-fa9c-88f7447b20ed_seg}.png} &
\includegraphics[width=.1595\textwidth]{images/results/{0.9354_sfo_df2a4d5e-6476-40f1-d0a9-898828e1593e_312de068-0f7b-407c-fa9c-88f7447b20ed_inf_pred}.png} &
\includegraphics[width=.1595\textwidth]{images/results/{0.9354_sfo_df2a4d5e-6476-40f1-d0a9-898828e1593e_312de068-0f7b-407c-fa9c-88f7447b20ed_inf_gt}.png} &\\

\includegraphics[width=.1595\textwidth]{images/results/{0.6456_sfo_39d06da9-25bc-40f1-d193-fc0564699aa4_4494d9f3-be3a-4ba3-d222-efd1b408af06_ground}.png} &
\includegraphics[width=.1595\textwidth]{images/results/{0.6456_sfo_39d06da9-25bc-40f1-d193-fc0564699aa4_4494d9f3-be3a-4ba3-d222-efd1b408af06_lidar}.png} &
\includegraphics[width=.1595\textwidth]{images/results/{0.6456_sfo_39d06da9-25bc-40f1-d193-fc0564699aa4_4494d9f3-be3a-4ba3-d222-efd1b408af06_dt}.png} &
\includegraphics[width=.1595\textwidth]{images/results/{0.6456_sfo_39d06da9-25bc-40f1-d193-fc0564699aa4_4494d9f3-be3a-4ba3-d222-efd1b408af06_seg}.png} &
\includegraphics[width=.1595\textwidth]{images/results/{0.6456_sfo_39d06da9-25bc-40f1-d193-fc0564699aa4_4494d9f3-be3a-4ba3-d222-efd1b408af06_inf_pred}.png} &
\includegraphics[width=.1595\textwidth]{images/results/{0.6456_sfo_39d06da9-25bc-40f1-d193-fc0564699aa4_4494d9f3-be3a-4ba3-d222-efd1b408af06_inf_gt}.png} &\\

\includegraphics[width=.1595\textwidth]{images/results/{0.9222_sfo_105a8b25-1edb-4317-c668-cff11cfd30b1_602a609c-7b42-47a2-c76a-f27b9a3708c2_ground}.png} &
\includegraphics[width=.1595\textwidth]{images/results/{0.9222_sfo_105a8b25-1edb-4317-c668-cff11cfd30b1_602a609c-7b42-47a2-c76a-f27b9a3708c2_lidar}.png} &
\includegraphics[width=.1595\textwidth]{images/results/{0.9222_sfo_105a8b25-1edb-4317-c668-cff11cfd30b1_602a609c-7b42-47a2-c76a-f27b9a3708c2_dt}.png} &
\includegraphics[width=.1595\textwidth]{images/results/{0.9222_sfo_105a8b25-1edb-4317-c668-cff11cfd30b1_602a609c-7b42-47a2-c76a-f27b9a3708c2_seg}.png} &
\includegraphics[width=.1595\textwidth]{images/results/{0.9222_sfo_105a8b25-1edb-4317-c668-cff11cfd30b1_602a609c-7b42-47a2-c76a-f27b9a3708c2_inf_pred}.png} &
\includegraphics[width=.1595\textwidth]{images/results/{0.9222_sfo_105a8b25-1edb-4317-c668-cff11cfd30b1_602a609c-7b42-47a2-c76a-f27b9a3708c2_inf_gt}.png} &\\

\includegraphics[width=.1595\textwidth]{images/results/{0.9188_sfo_402d89c7-06c2-4bb7-e2a0-000ebce602f3_78733220-cfbc-4b9e-c801-444d6dbdaca8_ground}.png} &
\includegraphics[width=.1595\textwidth]{images/results/{0.9188_sfo_402d89c7-06c2-4bb7-e2a0-000ebce602f3_78733220-cfbc-4b9e-c801-444d6dbdaca8_lidar}.png} &
\includegraphics[width=.1595\textwidth]{images/results/{0.9188_sfo_402d89c7-06c2-4bb7-e2a0-000ebce602f3_78733220-cfbc-4b9e-c801-444d6dbdaca8_dt}.png} &
\includegraphics[width=.1595\textwidth]{images/results/{0.9188_sfo_402d89c7-06c2-4bb7-e2a0-000ebce602f3_78733220-cfbc-4b9e-c801-444d6dbdaca8_seg}.png} &
\includegraphics[width=.1595\textwidth]{images/results/{0.9188_sfo_402d89c7-06c2-4bb7-e2a0-000ebce602f3_78733220-cfbc-4b9e-c801-444d6dbdaca8_inf_pred}.png} &
\includegraphics[width=.1595\textwidth]{images/results/{0.9188_sfo_402d89c7-06c2-4bb7-e2a0-000ebce602f3_78733220-cfbc-4b9e-c801-444d6dbdaca8_inf_gt}.png} &\\

a) & b) & c) & d) & e) & f) & \\
\end{tabular}

\caption{Offline map model results using the the model trained on both camera and LiDAR imagery). Comparisons between col a) input ground camera, b) input ground lidar, c) predicted inverse distance transform, d) predicted segmentation, e) our predicted crosswalk polygons after inference and f) ground truth crosswalk polygons.}
\label{fig:results}

\end{figure}

\begin{figure}
\begin{tabular}{cccccccr}
\includegraphics[width=.1595\textwidth]{images/results/{0.9314_sfo_1dc17567-83f7-4df3-f86e-78b86bd4283d_4890ccf8-901a-45f5-d135-6133cf5eaaf4_ground}.png} &
\includegraphics[width=.1595\textwidth]{images/results/{0.9314_sfo_1dc17567-83f7-4df3-f86e-78b86bd4283d_4890ccf8-901a-45f5-d135-6133cf5eaaf4_lidar}.png} &
\includegraphics[width=.1595\textwidth]{images/results/{0.9314_sfo_1dc17567-83f7-4df3-f86e-78b86bd4283d_4890ccf8-901a-45f5-d135-6133cf5eaaf4_dt}.png} &
\includegraphics[width=.1595\textwidth]{images/results/{0.9314_sfo_1dc17567-83f7-4df3-f86e-78b86bd4283d_4890ccf8-901a-45f5-d135-6133cf5eaaf4_seg}.png} &
\includegraphics[width=.1595\textwidth]{images/results/{0.9314_sfo_1dc17567-83f7-4df3-f86e-78b86bd4283d_4890ccf8-901a-45f5-d135-6133cf5eaaf4_inf_pred}.png} &
\includegraphics[width=.1595\textwidth]{images/results/{0.9314_sfo_1dc17567-83f7-4df3-f86e-78b86bd4283d_4890ccf8-901a-45f5-d135-6133cf5eaaf4_inf_gt}.png} &\\

\includegraphics[width=.1595\textwidth]{images/results/{0.9100_sfo_4d758bc6-687f-4fb0-e10c-b33bce8e4544_84d0333a-18b8-4ae6-f3ba-73027a3db5ab_ground}.png} &
\includegraphics[width=.1595\textwidth]{images/results/{0.9100_sfo_4d758bc6-687f-4fb0-e10c-b33bce8e4544_84d0333a-18b8-4ae6-f3ba-73027a3db5ab_lidar}.png} &
\includegraphics[width=.1595\textwidth]{images/results/{0.9100_sfo_4d758bc6-687f-4fb0-e10c-b33bce8e4544_84d0333a-18b8-4ae6-f3ba-73027a3db5ab_dt}.png} &
\includegraphics[width=.1595\textwidth]{images/results/{0.9100_sfo_4d758bc6-687f-4fb0-e10c-b33bce8e4544_84d0333a-18b8-4ae6-f3ba-73027a3db5ab_seg}.png} &
\includegraphics[width=.1595\textwidth]{images/results/{0.9100_sfo_4d758bc6-687f-4fb0-e10c-b33bce8e4544_84d0333a-18b8-4ae6-f3ba-73027a3db5ab_inf_pred}.png} &
\includegraphics[width=.1595\textwidth]{images/results/{0.9100_sfo_4d758bc6-687f-4fb0-e10c-b33bce8e4544_84d0333a-18b8-4ae6-f3ba-73027a3db5ab_inf_gt}.png} &\\

\includegraphics[width=.1595\textwidth]{images/results/{0.9317_sfo_dcaa19eb-862f-4ebf-c3f3-825876628416_aa2eb481-48c4-46a4-f445-0b459fbf3659_ground}.png} &
\includegraphics[width=.1595\textwidth]{images/results/{0.9317_sfo_dcaa19eb-862f-4ebf-c3f3-825876628416_aa2eb481-48c4-46a4-f445-0b459fbf3659_lidar}.png} &
\includegraphics[width=.1595\textwidth]{images/results/{0.9317_sfo_dcaa19eb-862f-4ebf-c3f3-825876628416_aa2eb481-48c4-46a4-f445-0b459fbf3659_dt}.png} &
\includegraphics[width=.1595\textwidth]{images/results/{0.9317_sfo_dcaa19eb-862f-4ebf-c3f3-825876628416_aa2eb481-48c4-46a4-f445-0b459fbf3659_seg}.png} &
\includegraphics[width=.1595\textwidth]{images/results/{0.9317_sfo_dcaa19eb-862f-4ebf-c3f3-825876628416_aa2eb481-48c4-46a4-f445-0b459fbf3659_inf_pred}.png} &
\includegraphics[width=.1595\textwidth]{images/results/{0.9317_sfo_dcaa19eb-862f-4ebf-c3f3-825876628416_aa2eb481-48c4-46a4-f445-0b459fbf3659_inf_gt}.png} &\\

\includegraphics[width=.1595\textwidth]{images/results/{0.8928_sfo_44cd0f5d-8553-4403-c910-a1b25c3a781d_9eab66d1-ceb7-41f2-f531-ab5b46a82108_ground}.png} &
\includegraphics[width=.1595\textwidth]{images/results/{0.8928_sfo_44cd0f5d-8553-4403-c910-a1b25c3a781d_9eab66d1-ceb7-41f2-f531-ab5b46a82108_lidar}.png} &
\includegraphics[width=.1595\textwidth]{images/results/{0.8928_sfo_44cd0f5d-8553-4403-c910-a1b25c3a781d_9eab66d1-ceb7-41f2-f531-ab5b46a82108_dt}.png} &
\includegraphics[width=.1595\textwidth]{images/results/{0.8928_sfo_44cd0f5d-8553-4403-c910-a1b25c3a781d_9eab66d1-ceb7-41f2-f531-ab5b46a82108_seg}.png} &
\includegraphics[width=.1595\textwidth]{images/results/{0.8928_sfo_44cd0f5d-8553-4403-c910-a1b25c3a781d_9eab66d1-ceb7-41f2-f531-ab5b46a82108_inf_pred}.png} &
\includegraphics[width=.1595\textwidth]{images/results/{0.8928_sfo_44cd0f5d-8553-4403-c910-a1b25c3a781d_9eab66d1-ceb7-41f2-f531-ab5b46a82108_inf_gt}.png} &\\

\includegraphics[width=.1595\textwidth]{images/results/{0.8823_sfo_1daf7b37-8455-4c82-d3b2-e299c41bce44_c4c7d0de-f8c9-4be6-faac-4cfec55e6e07_ground}.png} &
\includegraphics[width=.1595\textwidth]{images/results/{0.8823_sfo_1daf7b37-8455-4c82-d3b2-e299c41bce44_c4c7d0de-f8c9-4be6-faac-4cfec55e6e07_lidar}.png} &
\includegraphics[width=.1595\textwidth]{images/results/{0.8823_sfo_1daf7b37-8455-4c82-d3b2-e299c41bce44_c4c7d0de-f8c9-4be6-faac-4cfec55e6e07_dt}.png} &
\includegraphics[width=.1595\textwidth]{images/results/{0.8823_sfo_1daf7b37-8455-4c82-d3b2-e299c41bce44_c4c7d0de-f8c9-4be6-faac-4cfec55e6e07_seg}.png} &
\includegraphics[width=.1595\textwidth]{images/results/{0.8823_sfo_1daf7b37-8455-4c82-d3b2-e299c41bce44_c4c7d0de-f8c9-4be6-faac-4cfec55e6e07_inf_pred}.png} &
\includegraphics[width=.1595\textwidth]{images/results/{0.8823_sfo_1daf7b37-8455-4c82-d3b2-e299c41bce44_c4c7d0de-f8c9-4be6-faac-4cfec55e6e07_inf_gt}.png} &\\

\includegraphics[width=.1595\textwidth]{images/results/{0.1345_sfo_723289c4-0740-4a22-dd8d-1355216b0cf5_4ab0acfe-1ffb-403e-f3ea-2989c73680d3_ground}.png} &
\includegraphics[width=.1595\textwidth]{images/results/{0.1345_sfo_723289c4-0740-4a22-dd8d-1355216b0cf5_4ab0acfe-1ffb-403e-f3ea-2989c73680d3_lidar}.png} &
\includegraphics[width=.1595\textwidth]{images/results/{0.1345_sfo_723289c4-0740-4a22-dd8d-1355216b0cf5_4ab0acfe-1ffb-403e-f3ea-2989c73680d3_dt}.png} &
\includegraphics[width=.1595\textwidth]{images/results/{0.1345_sfo_723289c4-0740-4a22-dd8d-1355216b0cf5_4ab0acfe-1ffb-403e-f3ea-2989c73680d3_seg}.png} &
\includegraphics[width=.1595\textwidth]{images/results/{0.1345_sfo_723289c4-0740-4a22-dd8d-1355216b0cf5_4ab0acfe-1ffb-403e-f3ea-2989c73680d3_inf_pred}.png} &
\includegraphics[width=.1595\textwidth]{images/results/{0.1345_sfo_723289c4-0740-4a22-dd8d-1355216b0cf5_4ab0acfe-1ffb-403e-f3ea-2989c73680d3_inf_gt}.png} &\\

\includegraphics[width=.1595\textwidth]{images/results/{0.9617_sfo_7548b7a3-ef40-4208-c269-9235978ce767_6fe58a0d-f23c-4711-feef-f638d1978bcb_ground}.png} &
\includegraphics[width=.1595\textwidth]{images/results/{0.9617_sfo_7548b7a3-ef40-4208-c269-9235978ce767_6fe58a0d-f23c-4711-feef-f638d1978bcb_lidar}.png} &
\includegraphics[width=.1595\textwidth]{images/results/{0.9617_sfo_7548b7a3-ef40-4208-c269-9235978ce767_6fe58a0d-f23c-4711-feef-f638d1978bcb_dt}.png} &
\includegraphics[width=.1595\textwidth]{images/results/{0.9617_sfo_7548b7a3-ef40-4208-c269-9235978ce767_6fe58a0d-f23c-4711-feef-f638d1978bcb_seg}.png} &
\includegraphics[width=.1595\textwidth]{images/results/{0.9617_sfo_7548b7a3-ef40-4208-c269-9235978ce767_6fe58a0d-f23c-4711-feef-f638d1978bcb_inf_pred}.png} &
\includegraphics[width=.1595\textwidth]{images/results/{0.9617_sfo_7548b7a3-ef40-4208-c269-9235978ce767_6fe58a0d-f23c-4711-feef-f638d1978bcb_inf_gt}.png} &\\

\includegraphics[width=.1595\textwidth]{images/results/{0.9240_sfo_24f4a0ee-73f0-408a-f5da-6ec29c25980c_1b3fce76-64f5-49ad-c494-0d3a922320e5_ground}.png} &
\includegraphics[width=.1595\textwidth]{images/results/{0.9240_sfo_24f4a0ee-73f0-408a-f5da-6ec29c25980c_1b3fce76-64f5-49ad-c494-0d3a922320e5_lidar}.png} &
\includegraphics[width=.1595\textwidth]{images/results/{0.9240_sfo_24f4a0ee-73f0-408a-f5da-6ec29c25980c_1b3fce76-64f5-49ad-c494-0d3a922320e5_dt}.png} &
\includegraphics[width=.1595\textwidth]{images/results/{0.9240_sfo_24f4a0ee-73f0-408a-f5da-6ec29c25980c_1b3fce76-64f5-49ad-c494-0d3a922320e5_seg}.png} &
\includegraphics[width=.1595\textwidth]{images/results/{0.9240_sfo_24f4a0ee-73f0-408a-f5da-6ec29c25980c_1b3fce76-64f5-49ad-c494-0d3a922320e5_inf_pred}.png} &
\includegraphics[width=.1595\textwidth]{images/results/{0.9240_sfo_24f4a0ee-73f0-408a-f5da-6ec29c25980c_1b3fce76-64f5-49ad-c494-0d3a922320e5_inf_gt}.png} &\\

a) & b) & c) & d) & e) & f) & \\
\end{tabular}

\caption{Offline map model results using the the model trained on both camera and LiDAR imagery). Comparisons between col a) input ground camera, b) input ground lidar, c) predicted inverse distance transform, d) predicted segmentation, e) our predicted crosswalk polygons after inference and f) ground truth crosswalk polygons.}
\label{fig:results}

\end{figure}
